# Supplementary material for: Compressed Gradient Methods with Hessian-Aided Error Compensation
Source: arXiv:1909.10327 source file (2020-06-18)
Supplement: Supplementary file 1 [file appendix_cgd.tex]

% appendix_cgd
%%%%%%%%%%%%%%%%%%%%%%%%%%%%%%%%%%%%%%%%%%%%%%%%%%%%%
% Theorems: CGD 
%%%%%%%%%%%%%%%%%%%%%%%%%%%%%%%%%%%%%%%%%%%%%%%%%%%%%

%-------------------------------------------------------------------------------------------------------------------------------------------
%-------------------------------------------------------------------------------------------------------------------------------------------
% Theorem: CGD + convex
%-------------------------------------------------------------------------------------------------------------------------------------------
%-------------------------------------------------------------------------------------------------------------------------------------------
\section{Proof of Theorem \ref{thm:CGD_convex}}\label{app:thm:CGD_convex}
By the first property of UBEC,  $\mathbf{E} Q(\nabla f(x)) = \nabla f(x)$. In addition, by Lemma \ref{lemma:norm_sq_trick}, by the second property of UBEC, and by the Lipschitz smoothness of the whole objective function $f$, i.e. $\| \nabla f(x)\|^2\leq L\cdot \langle \nabla f(x) - \nabla f(x^\star), x-x^\star \rangle$ for $x\in\mathbb{R}^d$, we have: 
\begin{align*}
\mathbf{E}\| Q( \nabla f(x) ) \|^2 \leq 2L\cdot \mathbf{E}\langle \nabla f(x) - \nabla f(x^\star), x-x^\star \rangle + 2\epsilon.
\end{align*}
Therefore, we can easily prove Theorem  \ref{thm:CGD_convex} by Lemma \ref{lemma:Convex_C} with $\alpha_1=2L$ and $\alpha_2=2\epsilon$.

%-------------------------------------------------------------------------------------------------------------------------------------------
%-------------------------------------------------------------------------------------------------------------------------------------------
% Theorem: CGD + non-convex
%-------------------------------------------------------------------------------------------------------------------------------------------
%-------------------------------------------------------------------------------------------------------------------------------------------
\section{Proof of Theorem \ref{thm:CGD_nonconvex}}\label{app:thm:CGD_nonconvex}
By the first property of UBEC, $\mathbf{E} Q(\nabla f(x)) = \nabla f(x)$. In addition, by Lemma \ref{lemma:norm_sq_trick}, we have: 
\begin{align*}
\mathbf{E} \| Q(\nabla f(x)) \|^2 \leq 2 \mathbf{E}\| \nabla f(x) \|^2 + 2\epsilon. 
\end{align*}
Thus, we can easily prove Theorem \ref{thm:CGD_nonconvex} by applying Lemma \ref{lemma:NonConvex_C} with $\alpha_1=2$ and $\alpha_2=2\epsilon.$

%-------------------------------------------------------------------------------------------------------------------------------------------
%-------------------------------------------------------------------------------------------------------------------------------------------
% Theorem: ECCGD + convex
%-------------------------------------------------------------------------------------------------------------------------------------------
%-------------------------------------------------------------------------------------------------------------------------------------------
\section{Proof of Theorem \ref{thm:ECCGD_convex}}\label{app:thm:ECCGD_convex}
The equivalent EC-CGD update \eqref{eqn:ECCGD} is 
\begin{align}\label{eqn:ECCGDequivalent}
\tilde x_{k+1} = \tilde x_k - \gamma \nabla f(x_k),
\end{align}
where $\tilde x_k = x_k - \gamma e_k$. Thus, $\mathbf{E}\| \tilde x_k - x_k \|^2 = \gamma^2\mathbf{E}\|e_k\|^2 \leq \gamma^2\epsilon$ by the second property of UBEC. Therefore, we can easily prove Theorem \ref{thm:ECCGD_convex}
by Lemma \ref{lemma:Convex_EC} with $\theta=2L$, $\beta=\gamma^2\epsilon$, $\alpha_1=L$ and $\alpha_2=0$ (by the coercitivity of the 
whole objective function $f$).

%-------------------------------------------------------------------------------------------------------------------------------------------
%-------------------------------------------------------------------------------------------------------------------------------------------
% Theorem: ECCGD + non-convex
%-------------------------------------------------------------------------------------------------------------------------------------------
%-------------------------------------------------------------------------------------------------------------------------------------------
\section{Proof of Theorem \ref{thm:ECCGD_nonconvex}}\label{app:thm:ECCGD_nonconvex}
From the equivalent update of EC-CGD \eqref{eqn:ECCGDequivalent} and by the fact that $\mathbf{E}\| \tilde x_k - x_k \|^2 \leq \gamma^2\epsilon$ by the second property of UBEC, we prove Theorem \ref{thm:ECCGD_nonconvex}
by Lemma \ref{lemma:NonConvex_EC} with $\beta=\gamma^2\epsilon$, $\alpha_1=1$ and $\alpha_2=0$.
