# Supplementary material for: Compressed Gradient Methods with Hessian-Aided Error Compensation
Source: arXiv:1909.10327 source file (2020-06-18)
Supplement: Supplementary file 2 [file appendix_csgd.tex]

%%%%%%%%%%%%%%%%%%%%%%%%%%%%%%%%%%%%%%%%%
%%%%%%%%%%%%%%%%%%%%%%%%%%%%%%%%%%%%%%%%%
%====================================================%
% Theoretical results of Compressed SGD 
%====================================================%
%%%%%%%%%%%%%%%%%%%%%%%%%%%%%%%%%%%%%%%%%
%%%%%%%%%%%%%%%%%%%%%%%%%%%%%%%%%%%%%%%%%

%====================================================%
%====================================================%
% Theorem of Compressed SGD for convex optimization 
%====================================================%
%====================================================%
\section{Proof of Theorem \ref{thm:CSGD_convex}}\label{app:thm:CSGD_convex}
We start by stating one necessary lemma in our analysis. 
\begin{lemma}\label{lemma:CSGD_convex}
Assume that each loss function $f_i$ satisfies Assumptions \ref{assum:f_iLipsmooth} and \ref{assum:fiConvex}, and the compressor $Q$ is UBEC. Then, 
\begin{align*}
\mathbf{E}\left\| Q(\nabla f_{i_k}(x_k)) \right\|^2 \leq 3L \cdot \mathbf{E}\langle \nabla f(x_k) - \nabla f(x^\star), x_k-x^\star \rangle +  3( \epsilon + N),
\end{align*} 
where $N = {\max}_{i} \mathbf{E}\| \nabla f_i(x^\star)\|^2$.
\end{lemma}
\begin{proof}
By Lemma \ref{lemma:norm_sq_trick}, we have 
\begin{align*}
\mathbf{E}\left\| Q(\nabla f_{i_k}(x_k)) \right\|^2 \leq 3\mathbf{E}\left\| Q(\nabla f_{i_k}(x_k)) - \nabla f_{i_k}(x_k) \right\|^2 + 3\mathbf{E}\left\| \nabla f_{i_k}(x_k) - \nabla f_{i_k}(x^\star) \right\|^2 +  3\mathbf{E}\left\| \nabla f_{i_k}(x^\star) \right\|^2.
\end{align*}
Assume that $\mathbf{E}\| \nabla f_{i_k}(x^\star) \|^2 \leq N$. By the second property of UBEC, we get 
\begin{align*}
\mathbf{E}\left\| Q(\nabla f_{i_k}(x_k)) \right\|^2 \leq 3\mathbf{E}\left\| \nabla f_{i_k}(x_k) - \nabla f_{i_k}(x^\star) \right\|^2 +  3( \epsilon + N).
\end{align*}
Since $f_i$ is convex and $L-$smooth, 
\begin{align}\label{eqn:f_iSerebroTrick}
\| \nabla f_i(x) - \nabla f_i(y) \|^2 \leq L \langle \nabla f_i(x) - \nabla f_i(y), x-y \rangle, \quad \forall x,y\in\mathbb{R}^d.
\end{align}
Taking the expectation over the randomness yields 
\begin{equation}\label{eqn:f_iSerebro_mainTrick}
\begin{split}
\mathbf{E}\| \nabla f_{i_k}(x) - \nabla f_{i_k}(y) \|^2 
& \leq L \mathbf{E}\langle \nabla f_{i_k}(x) - \nabla f_{i_k}(y), x-y \rangle  \\ 
& \leq L \mathbf{E}\langle \nabla f(x) - \nabla f(y), x-y \rangle ,
\end{split}
\end{equation}
where the last inequality comes from the fact that $\mathbb{E}_{i_k} \nabla f_{i_k}(x) = \nabla f(x)$. Plugging this inequality with $x= x_k$ and $y = x^\star$ into the main result completes the proof. 
\end{proof}

Now, we are ready to prove Theorem \ref{thm:CSGD_convex}. By the fact that $\mathbf{E} \{ Q(\nabla f_{i_k}(x)) \}=\nabla f(x)$ and by Lemma \ref{lemma:CSGD_convex}, we have the convergence result of \eqref{eqn:CSGD} using  Lemma \ref{lemma:Convex_C} with $\alpha_1 = 3L$ and $\alpha_2 = 3(\epsilon + N)$. 

%====================================================%
%====================================================%
% Theorem of Compressed SGD for non-convex optimization 
%====================================================%
%====================================================%
\section{Proof of Theorem \ref{thm:CSGD_nonconvex}}\label{app:thm:CSGD_nonconvex}
Before deriving the main result, we provide the lemma which is useful in our analysis.
\begin{lemma}\label{lemma:CSGD_nonconvex}
Assume that each loss function $f_i$ satisfies Assumptions  \ref{assum:f_iLipsmooth} and 
 \ref{assum:fiBoundedVarNC}, and the compressor $Q$ is UBEC. Then,
 \begin{align*}
   \mathbf{E}\left\| Q(\nabla f_{i_k}(x_k)) \right\|^2 \leq  3\mathbf{E}\left\| \nabla f (x_k)  \right\|^2 +  3(\epsilon + \sigma^2).
 \end{align*} 
\end{lemma}
\begin{proof}
By Lemma \ref{lemma:norm_sq_trick}, we have 
\begin{align*}
\mathbf{E}\left\| Q(\nabla f_{i_k}(x_k)) \right\|^2 \leq 3\mathbf{E}\left\| Q(\nabla f_{i_k}(x_k)) - \nabla f_{i_k}(x_k) \right\|^2 + 3\mathbf{E}\left\| \nabla f_{i_k}(x_k) - \nabla f (x_k) \right\|^2 +  3\mathbf{E}\left\| \nabla f(x_k) \right\|^2.
\end{align*}
By the second property of UBEC and Assumption \ref{assum:fiBoundedVarNC}, we complete the proof. 
\end{proof} 

Now, we prove the main result. By the fact that $\mathbf{E} \left\{  Q (\nabla f_{i_k}(x)  )\right\} = \nabla f(x)$ and by Lemma \ref{lemma:CSGD_nonconvex}, we establish the main result of \eqref{eqn:CSGD} using Lemma \ref{lemma:NonConvex_C} with $\alpha_1=3$ and $\alpha_2 = 3(\epsilon +\sigma^2).$

%====================================================%
%====================================================%
% Theorem of Error-compressed SGD for convex optimization 
%====================================================%
%====================================================%
\section{Proof of Theorem \ref{thm:ECCSGD_convex}}\label{app:thm:ECCSGD_convex}
Before proving Theorem \ref{thm:ECCSGD_convex}, we introduce one important lemma. 
\begin{lemma}\label{lemma:ECCSGD_convex}
Assume that each loss function $f_i$ satisfies Assumptions \ref{assum:f_iLipsmooth} and \ref{assum:fiConvex}. Then, 
\begin{align*}
\mathbf{E}\left\| \nabla f_{i_k}(x_k) \right\|^2 \leq 2L \cdot \mathbf{E}\langle \nabla f(x_k) - \nabla f(x^\star), x_k-x^\star \rangle +  2N,
\end{align*} 
where $N = {\max}_{i} \mathbf{E}\| \nabla f_i(x^\star)\|^2$ and $\theta>0$.
\end{lemma}
\begin{proof}
By Lemma \ref{lemma:norm_sq_theta_trick}, we have 
\begin{align*}
\mathbf{E}\left\| \nabla f_{i_k}(x_k) \right\|^2 \leq  (1+\theta)\mathbf{E}\left\| \nabla f_{i_k}(x_k) - \nabla f_{i_k}(x^\star) \right\|^2 +  (1+1/\theta)\mathbf{E}\left\| \nabla f_{i_k}(x^\star) \right\|^2.
\end{align*}
Assume that $\mathbf{E}\| \nabla f_{i_k}(x^\star) \|^2 \leq N$ and $\theta=1$. Plugging
\eqref{eqn:f_iSerebro_mainTrick} due to convexity and smoothnes of $f_i$ into the main result completes the proof.   
\end{proof}

Now, we are ready to prove Theorem \eqref{lemma:ECCSGD_convex}. Define $\tilde x_k = x_k - \gamma e_k$. Then, the EC-CSGD update \eqref{eqn:EC-CSGD} can be re-written as 
\begin{align}\label{eqn:EC-CSGD_equi}
 \tilde x_{k+1} = \tilde x_k - \gamma \nabla f_{i_k}(x_k).
\end{align}
Also, it is easy to show that $\mathbf{E}\|x_k - \tilde x_k\|^2=\gamma^2 \mathbf{E}\|e_k\|^2=\gamma^2\epsilon$ by the second property of UBEC. By the unbiased property of $\nabla f_i$ and by Lemma \ref{lemma:ECCSGD_convex}, we establish the convergence rate result of \eqref{eqn:EC-CSGD} using Lemma \ref{lemma:Convex_EC} with $\alpha_1 = 2L$, $\alpha_2= 2N$, $\beta=\gamma^2\epsilon$ and $\theta=3L$.
%
%
%
%
%
%====================================================%
%====================================================%
% Theorem of Error-compressed SGD for non-convex optimization 
%====================================================%
%====================================================%
\section{Proof of Theorem \ref{thm:ECCSGD_nonconvex}}  \label{app:thm:ECCSGD_nonconvex}
Let us start by introducing one useful lemma for our analysis. 
\begin{lemma}\label{lemma:ECCSGD_nonconvex}
Let Assumption \ref{assum:fiBoundedVarNC} holds. Then, 
\begin{align*}
\mathbf{E}\| \nabla f_{i_k}(x_k) \|^2 \leq (1+\theta)\mathbf{E}\| \nabla f(x_k) \|^2 + (1+1/\theta)\sigma^2
\end{align*}
for $\theta>0.$
\end{lemma}
\begin{proof}
By Lemma \ref{lemma:norm_sq_theta_trick}, we have 
\begin{align*}
\mathbf{E}\| \nabla f_{i_k}(x_k) \|^2 \leq (1+\theta)\mathbf{E}\| \nabla f(x_k) \|^2 + (1+1/\theta)\mathbf{E}\| \nabla f_{i_k}(x_k) - \nabla f(x_k) \|^2.
\end{align*}
By Assumption \ref{assum:fiBoundedVarNC}, we obtain the result. 
\end{proof}
Now, we are ready to prove Theorem  \ref{thm:ECCSGD_nonconvex}. Define $\tilde x_k = x_k + \gamma e_k$. Then, the EC-CSGD equivalent update \eqref{eqn:EC-CSGD} is \eqref{eqn:EC-CSGD_equi}. Again, $\mathbf{E}\|x_k - \tilde x_k\|^2=\gamma^2 \mathbf{E}\|e_k\|^2=\gamma^2\epsilon$. By the unbiased property of $\nabla f_i$ and by Lemma \ref{lemma:ECCSGD_nonconvex}, we establish the convergence rate result of \eqref{eqn:EC-CSGD} using Lemma \ref{lemma:NonConvex_EC} with $\alpha_1 = 1+\theta$, $\alpha_2= (1+1/\theta)\sigma^2$, $\beta=\gamma^2\epsilon$ and $\theta=1/2$.
