# Supplementary material for: Compressed Gradient Methods with Hessian-Aided Error Compensation
Source: arXiv:1909.10327 source file (2020-06-18)
Supplement: Supplementary file 3 [file appendix_dist_csgd.tex]

%%%%%%%%%%%%%%%%%%%%%%%%%%%%%%%%%%%%%%
%%%%%%%%%%%%%%%%%%%%%%%%%%%%%%%%%%%%%%
% Theoretical results of distributed compressed gradient descent 
%%%%%%%%%%%%%%%%%%%%%%%%%%%%%%%%%%%%%%
%%%%%%%%%%%%%%%%%%%%%%%%%%%%%%%%%%%%%%

%================================================%
%================================================%
% dist CSGD: Convex
%================================================%
%================================================%
\section{Proof of Theorem \ref{thm:distCSGD_convex}}\label{app:thm:distCSGD_convex}
We start by introducing three important lemmas for our analysis.
\begin{lemma}\label{lemma:TrickBoundedError}
Let $Q$ be UBEC. Then, 
\begin{align*}
\mathbf{E}\left\| \frac{1}{m}\sum_{i=1}^m Q(g_i) - g_i \right\|^2 \leq \epsilon, \quad \forall g_i \in\mathbb{R}^d.
\end{align*}
\end{lemma}
\begin{proof}
We can easily prove this inequality by Lemma \ref{lemma:norm_sq_trick}, and by the second property of UBEC, i.e. $\mathbf{E}\|Q(v)-v\|^2\leq \epsilon$ for $v\in\mathbb{R}^d$ and $\epsilon>0$.
\end{proof}

\begin{lemma}\label{lemma:Trickgismoothandconvex}
Let each $g_i(x;\xi_i)$ be convex and $L-$smooth for every realization of $\xi_i$. Then, 
\begin{align*}
\mathbf{E}\left\| \frac{1}{m}\sum_{i=1}^m  \nabla g_i(x;\xi_i) - \nabla g_i(x^\star;\xi_i)  \right\|^2 \leq L \cdot \mathbf{E} \langle \nabla f(x) - \nabla f(x^\star), x- x^\star \rangle.
\end{align*}
\end{lemma}
\begin{proof}
By Lemma \ref{lemma:norm_sq_trick}, 
\begin{align*}
\mathbf{E}\left\| \frac{1}{m}\sum_{i=1}^m  \nabla g_i(x;\xi_i) - \nabla g_i(x^\star;\xi_i)  \right\|^2 
&\leq \frac{1}{m} \sum_{i=1}^m \mathbf{E}\left\| \nabla g_i(x;\xi_i) - \nabla g_i(x^\star;\xi_i)  \right\|^2 \\
& \leq  \frac{1}{m} \sum_{i=1}^m L \cdot \mathbf{E}\langle \nabla g_i(x;\xi_i) - \nabla g_i(x^\star;\xi_i) , x - x^\star  \rangle,
\end{align*}
where the second inequality comes from the Lipschitz coercitivity of $g_i(x;\xi_i)$ for every realization $\xi_i$. Since $\mathbf{E} \nabla g_i(x;\xi_i)=\nabla f_i(x)$ and $f(x) = (1/m)\sum_{i=1}^m f_i(x)$, we complete the proof. 
\end{proof}

\begin{lemma}\label{lemma:distCSGD_convex}
Let each $g_i(x;\xi_i)$ be convex and $L-$smooth for every realization of $\xi_i$, and the compressor $Q$ be UBEC. Then,  
\begin{align*}
\mathbf{E}\left\| \frac{1}{m}\sum_{i=1}^m Q(\nabla g_i(x;\xi_i)) \right\|^2 \leq  3L \cdot \mathbf{E} \langle \nabla f(x) - \nabla f(x^\star), x- x^\star \rangle + 3(\epsilon + N), 
\end{align*}
where $N = \mathbf{E}\left\| (1/m)\sum_{i=1}^m  \nabla g_i(x^\star;\xi_i)  \right\|^2.$
\end{lemma}
\begin{proof}
By Lemma \ref{lemma:norm_sq_trick}, we have
\begin{align*}
\mathbf{E}\left\| \frac{1}{m}\sum_{i=1}^m Q(\nabla g_i(x;\xi_i)) \right\|^2
& \leq 3 T_1 + 3 T_2 + 3N, \intertext{where}
T_1 & = \mathbf{E}\left\| \frac{1}{m}\sum_{i=1}^m Q(\nabla g_i(x;\xi_i)) - \nabla g_i(x;\xi_i) \right\|^2, \\ 
T_2 &=  \mathbf{E}\left\| \frac{1}{m}\sum_{i=1}^m  \nabla g_i(x;\xi_i) - \nabla g_i(x^\star;\xi_i)  \right\|^2, \quad \text{and} \\ 
N & = \mathbf{E}\left\| \frac{1}{m}\sum_{i=1}^m  \nabla g_i(x^\star;\xi_i)  \right\|^2. 
\end{align*} 
Substituting the inequalities of $T_1$ and $T_2$ from Lemmas \ref{lemma:TrickBoundedError} and \ref{lemma:Trickgismoothandconvex} yields the result.
\end{proof}

Now, we are ready to prove Theorem \ref{thm:distCSGD_convex}. By the fact that $\mathbf{E} \left\{ (1/m)\sum_{i=1}^m Q(\nabla g_i(x;\xi_i)) \right\} = \nabla f(x)$ and by Lemma \ref{lemma:distCSGD_convex}, we can prove Theorem \ref{thm:distCSGD_convex} using Lemma \ref{lemma:Convex_C} with $\alpha_1 = 3L$ and $\alpha_2 = 3(\epsilon+N)$.

%================================================%
%================================================%
% dist CSGD: Non-Convex
%================================================%
%================================================%
\section{Proof of Theorem \ref{thm:distCSGD_nonconvex}}\label{app:thm:distCSGD_nonconvex}
Before proving Theorem \ref{thm:distCSGD_nonconvex}, we introduce two important lemmas. 
\begin{lemma}\label{lemma:Trickgismooth_nonconvex}
Let Assumptions  \ref{assum:LonGi} and \ref{assum:GiBoundedVariance} hold. Then, 
\begin{align*}
\mathbf{E} \left\| \frac{1}{m}\sum_{i=1}^m \nabla g_i(x;\xi_i) - \nabla f_i(x) \right\|^2 \leq \sigma^2.
\end{align*}
\end{lemma}
\begin{proof}
The result can be easily obtained by Lemma \ref{lemma:norm_sq_trick}, and Assumption \ref{assum:GiBoundedVariance}.
\end{proof}

\begin{lemma}\label{lemma:distCSGD_nonconvex}
Let Assumptions  \ref{assum:LonGi} and \ref{assum:GiBoundedVariance} hold, and let the compressor $Q$ be UBEC. Then, 
\begin{align*}
\mathbf{E}\left\| \frac{1}{m}\sum_{i=1}^m Q(\nabla g_i(x;\xi_i)) \right\|^2 \leq 3\mathbf{E}\| \nabla f(x)\|^2 + 3(\epsilon +\sigma^2).
\end{align*}
\end{lemma}
\begin{proof}
By Lemma \ref{lemma:norm_sq_trick}, and by the fact that $f(x)=(1/m)\sum_{i=1}^m f_i(x)$, we obtain 
\begin{align*}
\mathbf{E}\left\| \frac{1}{m}\sum_{i=1}^m Q(\nabla g_i(x;\xi_i)) \right\|^2 & \leq 3T_1 + 3 T_2 + 3\mathbf{E}\| \nabla f(x) \|^2, \intertext{where} 
T_1 & = \mathbf{E}\left\| \frac{1}{m}\sum_{i=1}^m Q(\nabla g_i(x;\xi_i)) - \nabla g_i(x;\xi_i) \right\|^2 \\
T_2& = \mathbf{E}\left\| \frac{1}{m}\sum_{i=1}^m \nabla g_i(x;\xi_i) -\nabla f_i(x) \right\|^2.
\end{align*}
Using Lemmas \ref{lemma:TrickBoundedError} and \ref{lemma:Trickgismooth_nonconvex} yields the result. 
\end{proof}

Now, we can derive the main result. By the fact that $\mathbf{E} \left\{ (1/m)\sum_{i=1}^m Q(\nabla g_i(x;\xi_i)) \right\} = \nabla f(x)$ and by Lemma \ref{lemma:distCSGD_nonconvex}, we reach the result using Lemma \ref{lemma:NonConvex_C} with $\alpha_1 = 3$ and $\alpha_2 = 3(\epsilon+\sigma^2)$.

%================================================%
%================================================%
% dist EC-CSGD: Convex
%================================================%
%================================================%
\section{Proof of Theorem \ref{thm:distEC-CSGD_convex}}\label{app:thm:distEC-CSGD_convex}
To prove Theorem \ref{thm:distEC-CSGD_convex}, we start by providing one important lemma for our analysis. 
\begin{lemma} \label{lemma:distEC-CSGD_convex}
Let each $g_i(x;\xi_i)$ be convex and $L-$smooth for every realization of $\xi_i$. Then, 
\begin{align*}
\mathbf{E} \left\| \frac{1}{m} \sum_{i=1}^m g_i(x;\xi_i) \right\|^2 \leq 2L\cdot\mathbf{E}\langle \nabla f(x) - \nabla f(x^\star), x - x^\star \rangle + 2 N,
\end{align*}
where $N = \mathbf{E} \left\| (1/m) \sum_{i=1}^m g_i(x^\star;\xi_i) \right\|^2.$
\end{lemma}
\begin{proof}
By Lemma \ref{lemma:norm_sq_trick}, we have 
\begin{align*}
\mathbf{E} \left\| \frac{1}{m} \sum_{i=1}^m g_i(x;\xi_i) \right\|^2 \leq 2  \mathbf{E} \left\| \frac{1}{m} \sum_{i=1}^m g_i(x;\xi_i) - g_i(x^\star;\xi_i) \right\|^2 + 2\mathbf{E} \left\| \frac{1}{m} \sum_{i=1}^m g_i(x^\star;\xi_i) \right\|^2. 
\end{align*}
Next, applying Lemmas \ref{lemma:TrickBoundedError} and \ref{lemma:Trickgismoothandconvex} into the main inequality completes the proof.
\end{proof}
Now, we are ready to prove Theorem \ref{thm:distEC-CSGD_convex}. Define $\tilde x_k = x_k - \gamma (1/m)\sum_{i=1}^m e_k^i$. Then, the equivalent update of D-EC-CSGD \eqref{eqn:DECCSGD} is 
\begin{align}
\tilde x_{k+1} = \tilde x_k -\gamma \frac{1}{m}\sum_{i=1}^m Q(\nabla g_i(x_k;\xi_i)).
\end{align}
In addition, we can show that $\mathbf{E}\| x_k - \tilde x_k \|^2=\gamma^2\mathbf{E}\| (1/m)\sum_{i=1}^m Q(\nabla g_i(x_k;\xi_i)) \|^2 \leq \gamma^2 \epsilon$ by Lemma \ref{lemma:TrickBoundedError}. By the fact that $\mathbf{E} \{(1/m)\sum_{i=1}^m \nabla g_i(x;\xi_i)\} = \nabla f(x)$ and by  Lemma \ref{lemma:distEC-CSGD_convex}, using Lemma \ref{lemma:Convex_EC} with $\alpha_1 = 2L, \alpha_2=2N, \beta = \gamma^2\epsilon$ and $\theta=3L$ completes the proof.

%================================================%
%================================================%
% dist EC-CSGD: Non-Convex
%================================================%
%================================================%
\section{Proof of Theorem \ref{thm:distEC-CSGD_nonconvex}
}\label{app:thm:distEC-CSGD_nonconvex}
We begin with providing one lemma which is necessary to prove Theorem \ref{thm:distEC-CSGD_nonconvex}. 
\begin{lemma}
Let Assumptions  \ref{assum:LonGi} and \ref{assum:GiBoundedVariance} hold. Then, 
\begin{align*}
\mathbf{E} \left\| \frac{1}{m}\sum_{i=1}^m \nabla g_i(x;\xi_i) \right\|^2 \leq (1+\theta)\mathbf{E}\| \nabla f(x) \|^2+(1+1/\theta)\sigma^2.
\end{align*}
\end{lemma}
\begin{proof}
We can easily reach the inequality by the fact that $\nabla f(x) = (1/m) \sum_{i=1}^m \nabla f_i(x)$, and by Lemmas \ref{lemma:norm_sq_theta_trick} and \ref{lemma:Trickgismooth_nonconvex}.
\end{proof}

Following the proof arguments in Theorem \ref{thm:distEC-CSGD_convex}, we prove Theorem  \ref{thm:distEC-CSGD_nonconvex} by Lemma \ref{lemma:NonConvex_EC} with $\alpha_1 = 1+\theta, \alpha_2 = (1+1/\theta)\sigma^2, \beta = \gamma^2\epsilon,$ and $\theta=1/2.$
