# Supplementary material for: Compressed Gradient Methods with Hessian-Aided Error Compensation
Source: arXiv:1909.10327 source file (2020-06-18)
Supplement: Supplementary file 4 [file appendix_dist_csgd_SK_1.tex]

%%%%%%%%%%%%%%%%%%%%%%%%%%%%%%%%%%%%%%
%%%%%%%%%%%%%%%%%%%%%%%%%%%%%%%%%%%%%%
% Theoretical results of distributed compressed gradient descent 
%%%%%%%%%%%%%%%%%%%%%%%%%%%%%%%%%%%%%%
%%%%%%%%%%%%%%%%%%%%%%%%%%%%%%%%%%%%%%

%================================================%
%================================================%
% dist CSGD
%================================================%
%================================================%

\section{Analysis of Algorithm \eqref{eqn:QDGD}}\label{app:distCSGD}

In this section, we analyze the convergence rate of D-CSGD \eqref{eqn:QDGD} for strongly convex and non-convex optimization. 
The equivalent update of D-CSGD \eqref{eqn:QDGD} is 
\begin{align}
x^{k+1} & = x^k - \gamma \left( \nabla f(x^k) +\eta^k + \omega^k + e^k \right), 
\intertext{where}
\omega ^k & = \frac{1}{n}\sum_{i=1}^n \omega_i^k \nonumber \\ 
\eta^k &=  \frac{1}{n}\sum_{i=1}^n \left[  \nabla g_i(x^k;\xi_i^k) - \nabla f_i(x^k)   \right], \quad \text{and} \nonumber \\ 
e^k & = \frac{1}{n}\sum_{i=1}^n   \left[ Q\left( \nabla g_i(x^k;\xi_i^k) + \omega_i^k \right) - ( \nabla g_i(x^k;\xi_i^k) +\omega_i^k) \right]. \nonumber
\end{align}
Since $\mathbf{E} \omega_i^k = 0$ and $\mathbf{E}\|  \omega_i^k \|^2 \leq \sigma_\omega^2$, we easily prove that $\mathbf{E} \omega^k = 0$ and $\mathbf{E}\|  \omega^k \|^2 \leq \sigma_\omega^2$. Similarly, since $\mathbf{E} \nabla g_i(x^k;\xi_i^k) = \nabla f_i(x^k)$ and $\mathbf{E}\| \nabla g_i(x^k;\xi_i^k) - \nabla f_i(x^k)  \|^2 \leq \sigma_v^2$, it is easy to verify that $\mathbf{E} \eta^k =0$ and $\mathbf{E} \|\eta^k \|^2 \leq \sigma_v^2$. Finally, by the property of the $\epsilon-$compressor it is easy to derive that $\| e^k \|^2 \leq \epsilon^2$.

Therefore, we easily derive the convergence results of D-CSGD \eqref{eqn:QDGD} for strongly convex and non-convex optimization by following derivations from Theorems \ref{thm:CGD_SC} and \ref{thm:CGD_NC}, respectively.

\section{Analysis of Algorithm \eqref{eqn:DECCSGD}}\label{app:thm:distEC-CSGD}
In this section, we analyze the convergence rate of D-EC-CSGD \eqref{eqn:DECCSGD}  for strongly convex and non-convex optimization. Consider the case when $A_i^k = I -\gamma H_i^k$. Then, the equivalent update of D-EC-CSGD \eqref{eqn:DECCSGD} is 
\begin{align}
\tilde x^{k+1} &= \tilde x^k - \gamma \left[ \nabla f(x^k) +\eta^k + \omega^k \right] + \gamma^2 \frac{1}{n}\sum_{i=1}^n H_i^k e_i^k,
\intertext{where}
\tilde x^k &= x^k - \frac{1}{n}\sum_{i=1}^n e_i^k, \quad \text{and} \nonumber \\ 
\omega^k & = \frac{1}{n}\sum_{i=1}^n \omega_i^k \nonumber \\ 
\eta^k & =  \frac{1}{n}\sum_{i=1}^n \left[ \nabla g_i(x^k;\xi_i^k) - \nabla f_i(x^k) \right]
\end{align}
Following Section \ref{app:distCSGD}, it is easy to prove that $\mathbf{E} \omega^k =0$ and $\mathbf{E} \| \omega^k \|^2 \leq \sigma^2_\omega$, and $\mathbf{E} \eta^k=0$ and $\mathbf{E}\| \eta^k \|^2\leq \sigma^2_v$. In addition,  by the propertiy of the $\epsilon-$compressor and by the error compensation step we can easily verify that $\| (1/n) \sum_{i=1}^n e_i^k \|^2 \leq  \epsilon^2$.  Finally, if $H_i^k \preccurlyeq \Lambda I$, then $\| (1/n) \sum_{i=1}^n H_i^k e_i^k \|^2 \leq \Lambda^2 \epsilon^2$.

Following the derivations in Theorems \ref{thm:ECCSGD_SC} and \ref{thm:ECCSGD_NC}, we reach the convergence rate results of \eqref{eqn:DECCSGD} with $A_i^k = I -\gamma H_i^k$ for strongly convex and non-convex optimization, respectively. The main difference is that the terms related to $H^k e^k$ in these theorems are replaced by $(1/n) \sum_{i=1}^n H_i^k e_i^k $.
