# Supplementary material for: Compressed Gradient Methods with Hessian-Aided Error Compensation
Source: arXiv:1909.10327 source file (2020-06-18)
Supplement: Supplementary file 7 [file appendix_main.tex]

\documentclass[../main.tex]{subfiles}

\begin{document}
 \appendices
\input{Appendix/appendix_lemmas_SK_1}
\input{Appendix/appendix_cgd_SK_1}
\end{document}
